# Supplementary material for: Adversarial Robustness for Code
Source: arXiv:2002.04694 source file (2020-08-15)
Supplement: Supplementary file 3 [file supplementary.tex]

\appendix
\section{Evaluation}

\paragraph{Dataset}
To obtain the datasets used in our work we extend the infrastructure from \scode{DeepTyper}~\cite{DeepTyper:18}, collect the same top starred projects on Github, and perform similar preprocessing steps -- remove \scode{TypeScript} header files, remove files with less than 100 or more than 3,000 tokens and split the projects into train, validation and test datasets such that each project is fully contained in one of the datasets.
Additionally, we remove exact file duplicates and files that are similar to each other ($\approx\!10\%$ of the files). We measure file similarity by collecting all 3-grams (excluding comments and whitespace) and removing files with Jaccard similarity greater than~$0.7$.

We compute the ground-truth types using the \scode{TypeScript} compiler version $3.4.5$ based on manual type annotations, library specifications and analyzing all project files.
In contrast to the datasets used in \cite{DeepTyper:18}, we additionally include the types corresponding to all intermediate expressions and constants (e.g., the expression $x + y$ contains three predictions for $x$, $y$ and $x+y$).
This improves model performance as it is explicitly trained also on the intermediate steps required to infer the types.
We train all the models to predict four primitive types (\scode{string}, \scode{number}, \scode{boolean}, \scode{void}), four function types ($()\!\Rightarrow\!\scode{string}$, $()\!\Rightarrow\!\scode{number}$, $()\!\Rightarrow\!\scode{boolean}$, $()\!\Rightarrow\!\scode{void}$) and a~special \scode{unk} label denoting all the other~types.

\paragraph{Program modifications}
We instantiate adversarial training with the following types of program modifications -- variable renaming, constant substitution, object field renaming (e.g., $\scode{obj.x}\!\rightarrow\!\scode{obj.y}$), property assignment renaming (e.g., $\{\scode{x}\colon \scode{obj}\} \rightarrow \{\scode{y}\colon \scode{obj}\}$) and wrapping expressions, variables and constants in a ternary operator (e.g., $\scode{x} \rightarrow (\scode{expr}) : \scode{x}~?~\scode{x}$). Here, $\scode{expr}$ is effectively a dead code and consists of a~random binary expression over constants up to depth 3.

Furthermore, during adversarial training, if multiple $\mods$ lead to mis-classification, we train on all of them and not only on the one that leads to the highest loss.

\paragraph{Effect of dataset size}
All results presented in \Tabrefs{baseline_accuracy} and \ref{Ta:breakdown} are obtained by training our models using a dataset that contains 3000 programs split equally between training, validation and test datasets.
As described earlier, the effective training dataset size is in practice up to two orders of magnitude larger as the adversarial training considers a larger dataset obtained by applying valid modifications $\Delta(x)$ to the dataset~$\dataset$.
However, a natural question is -- how does dataset size affect model accuracy and  robustness?
To answer this question, we trained our models with a 10 times larger initial training dataset containing 10,000 programs, while keeping the validation and test dataset the same.

For all models, increasing dataset size leads to the results consistent with those presented so far, except that both accuracy and robustness improve by $\approx\!3\%$ and up to $\approx\!2\%$, respectively.
Concretely, the \gnn{} accuracy improves from $89.33\%$ to $93.36\%$ and from $90.30\%$ to $93.41\%$ when using standard and adversarial training, respectively.
The \gnn{} robustness slightly decreases for standard training from $54.86\%$ to $54.37\%$ but improves from $54.40\%$ to $56.92\%$ when using adversarial training.
This shows that using a large and diverse input dataset is important for achieving high accuracy, but it is insufficient for achieving model robustness, a problem our method addresses.
